# Supplementary material for: Estimation of Spectral Biophysical Skin Properties from Captured RGB Albedo
Source: arXiv:2201.10695 source file (2022-01-26)
Supplement: Supplementary file 1 [file neuraldiff.tex]

%\newpage
%\section{Neural Reconstruction difference images}
In Figure~\ref{fig:neuraldiff_1} - Figure~\ref{fig:neuraldiff_8}, we show the reconstruction $L_1$ difference images for all faces. We use the same masks as in computing the reconstruction loss and consider the difference to be zero in the non-skin regions. We observed that 150 $L_1 L_2$ and 200 $L_1 L2$ networks produce visually the  lowest errors.

\begin{figure*}
 \contourlength{0.1em}%
 \centering
 \hspace*{-4.5mm}%
  \begin{tabular}{l@{\;}c@{\;}c@{\;}c}
 & \textsc{L1} & \textsc{L2} & \textsc{L1L2} 
  \\
   \begin{sideways}\hspace{2cm}\textsc{50}\end{sideways}
  &
  \begin{overpic}[width=0.3\textwidth]{fig_supp/neuraldiff/50_L1_laure_reconstruction_diff.jpg}
  \end{overpic}
 &
  \begin{overpic}[width=0.3\textwidth]{fig_supp/neuraldiff/50_L2_laure_reconstruction_diff.jpg}
  \end{overpic}
  &
  \begin{overpic}[width=0.3\textwidth]{fig_supp/neuraldiff/50_L1L2_laure_reconstruction_diff.jpg}
  \end{overpic}
  \\
  \begin{sideways}\hspace{2cm}\textsc{100}\end{sideways}
  &
  \begin{overpic}[width=0.3\textwidth]{fig_supp/neuraldiff/100_L1_laure_reconstruction_diff.jpg}
  \end{overpic}
 &
  \begin{overpic}[width=0.3\textwidth]{fig_supp/neuraldiff/100_L2_laure_reconstruction_diff.jpg}
  \end{overpic}
  &
  \begin{overpic}[width=0.3\textwidth]{fig_supp/neuraldiff/100_L1L2_laure_reconstruction_diff.jpg}
  \end{overpic}
  \\
  \begin{sideways}\hspace{2cm}\textsc{150}\end{sideways}
  &
   \begin{overpic}[width=0.3\textwidth]{fig_supp/neuraldiff/150_L1_laure_reconstruction_diff.jpg}
  \end{overpic}
 &
  \begin{overpic}[width=0.3\textwidth]{fig_supp/neuraldiff/150_L2_laure_reconstruction_diff.jpg}
  \end{overpic}
  &
  \begin{overpic}[width=0.3\textwidth]{fig_supp/neuraldiff/150_L1L2_laure_reconstruction_diff.jpg}
  \end{overpic}
  \\
  \begin{sideways}\hspace{2cm}\textsc{200}\end{sideways}
  &
  \begin{overpic}[width=0.3\textwidth]{fig_supp/neuraldiff/200_L1_laure_reconstruction_diff.jpg}
  \end{overpic}
 &
  \begin{overpic}[width=0.3\textwidth]{fig_supp/neuraldiff/200_L2_laure_reconstruction_diff.jpg}
  \end{overpic}
  &
  \begin{overpic}[width=0.3\textwidth]{fig_supp/neuraldiff/200_L1L2_laure_reconstruction_diff.jpg}
  \end{overpic}
 \end{tabular}
 \vspace{-3mm}
%  \caption{Laure}
  \caption{Subject B - Type I}
  \label{fig:neuraldiff_1}
  \vspace{-6mm}
\end{figure*}

\begin{figure*}
 \contourlength{0.1em}%
 \centering
 \hspace*{-4.5mm}%
  \begin{tabular}{l@{\;}c@{\;}c@{\;}c}
 & \textsc{L1} & \textsc{L2} & \textsc{L1L2} 
  \\
   \begin{sideways}\hspace{1cm}\textsc{50}\end{sideways}
  &
  \begin{overpic}[width=0.3\textwidth]{fig_supp/neuraldiff/50_L1_whitefemale_reconstruction_diff.jpg}
  \end{overpic}
 &
  \begin{overpic}[width=0.3\textwidth]{fig_supp/neuraldiff/50_L2_whitefemale_reconstruction_diff.jpg}
  \end{overpic}
  &
  \begin{overpic}[width=0.3\textwidth]{fig_supp/neuraldiff/50_L1L2_whitefemale_reconstruction_diff.jpg}
  \end{overpic}
  \\
  \begin{sideways}\hspace{1cm}\textsc{100}\end{sideways}
  &
  \begin{overpic}[width=0.3\textwidth]{fig_supp/neuraldiff/100_L1_whitefemale_reconstruction_diff.jpg}
  \end{overpic}
 &
  \begin{overpic}[width=0.3\textwidth]{fig_supp/neuraldiff/100_L2_whitefemale_reconstruction_diff.jpg}
  \end{overpic}
  &
  \begin{overpic}[width=0.3\textwidth]{fig_supp/neuraldiff/100_L1L2_whitefemale_reconstruction_diff.jpg}
  \end{overpic}
  \\
  \begin{sideways}\hspace{1cm}\textsc{150}\end{sideways}
  &
   \begin{overpic}[width=0.3\textwidth]{fig_supp/neuraldiff/150_L1_whitefemale_reconstruction_diff.jpg}
  \end{overpic}
 &
  \begin{overpic}[width=0.3\textwidth]{fig_supp/neuraldiff/150_L2_whitefemale_reconstruction_diff.jpg}
  \end{overpic}
  &
  \begin{overpic}[width=0.3\textwidth]{fig_supp/neuraldiff/150_L1L2_whitefemale_reconstruction_diff.jpg}
  \end{overpic}
  \\
  \begin{sideways}\hspace{1cm}\textsc{200}\end{sideways}
  &
  \begin{overpic}[width=0.3\textwidth]{fig_supp/neuraldiff/200_L1_whitefemale_reconstruction_diff.jpg}
  \end{overpic}
 &
  \begin{overpic}[width=0.3\textwidth]{fig_supp/neuraldiff/200_L2_whitefemale_reconstruction_diff.jpg}
  \end{overpic}
  &
  \begin{overpic}[width=0.3\textwidth]{fig_supp/neuraldiff/200_L1L2_whitefemale_reconstruction_diff.jpg}
  \end{overpic}
 \end{tabular}
 \vspace{-3mm}
%  \caption{whitefemale}
  \caption{Subject B - Type I}
  \label{fig:neuraldiff_2}
  \vspace{-6mm}
\end{figure*}

\begin{figure*}
 \contourlength{0.1em}%
 \centering
 \hspace*{-4.5mm}%
  \begin{tabular}{l@{\;}c@{\;}c@{\;}c}
 & \textsc{L1} & \textsc{L2} & \textsc{L1L2} 
  \\
  \begin{sideways}\hspace{2cm}\textsc{50}\end{sideways}
  &
  \begin{overpic}[width=0.3\textwidth]{fig_supp/neuraldiff/50_L1_ronald_reconstruction_diff.jpg}
  \end{overpic}
 &
  \begin{overpic}[width=0.3\textwidth]{fig_supp/neuraldiff/50_L2_ronald_reconstruction_diff.jpg}
  \end{overpic}
  &
  \begin{overpic}[width=0.3\textwidth]{fig_supp/neuraldiff/50_L1L2_ronald_reconstruction_diff.jpg}
  \end{overpic}
  \\
  \begin{sideways}\hspace{2cm}\textsc{100}\end{sideways}
  &
  \begin{overpic}[width=0.3\textwidth]{fig_supp/neuraldiff/100_L1_ronald_reconstruction_diff.jpg}
  \end{overpic}
 &
  \begin{overpic}[width=0.3\textwidth]{fig_supp/neuraldiff/100_L2_ronald_reconstruction_diff.jpg}
  \end{overpic}
  &
  \begin{overpic}[width=0.3\textwidth]{fig_supp/neuraldiff/100_L1L2_ronald_reconstruction_diff.jpg}
  \end{overpic}
  \\
  \begin{sideways}\hspace{2cm}\textsc{150}\end{sideways}
  &
   \begin{overpic}[width=0.3\textwidth]{fig_supp/neuraldiff/150_L1_ronald_reconstruction_diff.jpg}
  \end{overpic}
 &
  \begin{overpic}[width=0.3\textwidth]{fig_supp/neuraldiff/150_L2_ronald_reconstruction_diff.jpg}
  \end{overpic}
  &
  \begin{overpic}[width=0.3\textwidth]{fig_supp/neuraldiff/150_L1L2_ronald_reconstruction_diff.jpg}
  \end{overpic}
  \\
  \begin{sideways}\hspace{2cm}\textsc{200}\end{sideways}
  &
  \begin{overpic}[width=0.3\textwidth]{fig_supp/neuraldiff/200_L1_ronald_reconstruction_diff.jpg}
  \end{overpic}
 &
  \begin{overpic}[width=0.3\textwidth]{fig_supp/neuraldiff/200_L2_ronald_reconstruction_diff.jpg}
  \end{overpic}
  &
  \begin{overpic}[width=0.3\textwidth]{fig_supp/neuraldiff/200_L1L2_ronald_reconstruction_diff.jpg}
  \end{overpic}
 \end{tabular}
 \vspace{-3mm}
%  \caption{Ronald}
  \caption{Subject C - Type II}
  \label{fig:neuraldiff_3}
  \vspace{-6mm}
\end{figure*}

\begin{figure*}
 \contourlength{0.1em}%
 \centering
 \hspace*{-4.5mm}%
  \begin{tabular}{l@{\;}c@{\;}c@{\;}c}
 & \textsc{L1} & \textsc{L2} & \textsc{L1L2} 
  \\
   \begin{sideways}\hspace{2cm}\textsc{50}\end{sideways}
  &
  \begin{overpic}[width=0.3\textwidth]{fig_supp/neuraldiff/50_L1_tony_reconstruction_diff.jpg}
  \end{overpic}
 &
  \begin{overpic}[width=0.3\textwidth]{fig_supp/neuraldiff/50_L2_tony_reconstruction_diff.jpg}
  \end{overpic}
  &
  \begin{overpic}[width=0.3\textwidth]{fig_supp/neuraldiff/50_L1L2_tony_reconstruction_diff.jpg}
  \end{overpic}
  \\
  \begin{sideways}\hspace{2cm}\textsc{100}\end{sideways}
  &
  \begin{overpic}[width=0.3\textwidth]{fig_supp/neuraldiff/100_L1_tony_reconstruction_diff.jpg}
  \end{overpic}
 &
  \begin{overpic}[width=0.3\textwidth]{fig_supp/neuraldiff/100_L2_tony_reconstruction_diff.jpg}
  \end{overpic}
  &
  \begin{overpic}[width=0.3\textwidth]{fig_supp/neuraldiff/100_L1L2_tony_reconstruction_diff.jpg}
  \end{overpic}
  \\
  \begin{sideways}\hspace{2cm}\textsc{150}\end{sideways}
  &
   \begin{overpic}[width=0.3\textwidth]{fig_supp/neuraldiff/150_L1_tony_reconstruction_diff.jpg}
  \end{overpic}
 &
  \begin{overpic}[width=0.3\textwidth]{fig_supp/neuraldiff/150_L2_tony_reconstruction_diff.jpg}
  \end{overpic}
  &
  \begin{overpic}[width=0.3\textwidth]{fig_supp/neuraldiff/150_L1L2_tony_reconstruction_diff.jpg}
  \end{overpic}
  \\
  \begin{sideways}\hspace{2cm}\textsc{200}\end{sideways}
  &
  \begin{overpic}[width=0.3\textwidth]{fig_supp/neuraldiff/200_L1_tony_reconstruction_diff.jpg}
  \end{overpic}
 &
  \begin{overpic}[width=0.3\textwidth]{fig_supp/neuraldiff/200_L2_tony_reconstruction_diff.jpg}
  \end{overpic}
  &
  \begin{overpic}[width=0.3\textwidth]{fig_supp/neuraldiff/200_L1L2_tony_reconstruction_diff.jpg}
  \end{overpic}
 \end{tabular}
 \vspace{-3mm}
%  \caption{Tony}
  \caption{Subject D - Type III}
  \label{fig:neuraldiff_4}
  \vspace{-6mm}
\end{figure*}

\begin{figure*}
 \contourlength{0.1em}%
 \centering
 \hspace*{-4.5mm}%
  \begin{tabular}{l@{\;}c@{\;}c@{\;}c}
 & \textsc{L1} & \textsc{L2} & \textsc{L1L2} 
  \\
    \begin{sideways}\hspace{2cm}\textsc{50}\end{sideways}
  &
  \begin{overpic}[width=0.3\textwidth]{fig_supp/neuraldiff/50_L1_yaser_reconstruction_diff.jpg}
  \end{overpic}
 &
  \begin{overpic}[width=0.3\textwidth]{fig_supp/neuraldiff/50_L2_yaser_reconstruction_diff.jpg}
  \end{overpic}
  &
  \begin{overpic}[width=0.3\textwidth]{fig_supp/neuraldiff/50_L1L2_yaser_reconstruction_diff.jpg}
  \end{overpic}
  \\
  \begin{sideways}\hspace{2cm}\textsc{100}\end{sideways}
  &
  \begin{overpic}[width=0.3\textwidth]{fig_supp/neuraldiff/100_L1_yaser_reconstruction_diff.jpg}
  \end{overpic}
 &
  \begin{overpic}[width=0.3\textwidth]{fig_supp/neuraldiff/100_L2_yaser_reconstruction_diff.jpg}
  \end{overpic}
  &
  \begin{overpic}[width=0.3\textwidth]{fig_supp/neuraldiff/100_L1L2_yaser_reconstruction_diff.jpg}
  \end{overpic}
  \\
  \begin{sideways}\hspace{2cm}\textsc{150}\end{sideways}
  &
   \begin{overpic}[width=0.3\textwidth]{fig_supp/neuraldiff/150_L1_yaser_reconstruction_diff.jpg}
  \end{overpic}
 &
  \begin{overpic}[width=0.3\textwidth]{fig_supp/neuraldiff/150_L2_yaser_reconstruction_diff.jpg}
  \end{overpic}
  &
  \begin{overpic}[width=0.3\textwidth]{fig_supp/neuraldiff/150_L1L2_yaser_reconstruction_diff.jpg}
  \end{overpic}
  \\
  \begin{sideways}\hspace{2cm}\textsc{200}\end{sideways}
  &
  \begin{overpic}[width=0.3\textwidth]{fig_supp/neuraldiff/200_L1_yaser_reconstruction_diff.jpg}
  \end{overpic}
 &
  \begin{overpic}[width=0.3\textwidth]{fig_supp/neuraldiff/200_L2_yaser_reconstruction_diff.jpg}
  \end{overpic}
  &
  \begin{overpic}[width=0.3\textwidth]{fig_supp/neuraldiff/200_L1L2_yaser_reconstruction_diff.jpg}
  \end{overpic}
 \end{tabular}
 \vspace{-3mm}
%  \caption{Yaser}
  \caption{Subject E - Type IV}
  \label{fig:neuraldiff_5}
  \vspace{-6mm}
\end{figure*}

\begin{figure*}
 \contourlength{0.1em}%
 \centering
 \hspace*{-4.5mm}%
  \begin{tabular}{l@{\;}c@{\;}c@{\;}c}
 & \textsc{L1} & \textsc{L2} & \textsc{L1L2} 
  \\
   \begin{sideways}\hspace{2cm}\textsc{50}\end{sideways}
  &
  \begin{overpic}[width=0.3\textwidth]{fig_supp/neuraldiff/50_L1_dinora_reconstruction_diff.jpg}
  \end{overpic}
 &
  \begin{overpic}[width=0.3\textwidth]{fig_supp/neuraldiff/50_L2_dinora_reconstruction_diff.jpg}
  \end{overpic}
  &
  \begin{overpic}[width=0.3\textwidth]{fig_supp/neuraldiff/50_L1L2_dinora_reconstruction_diff.jpg}
  \end{overpic}
  \\
  \begin{sideways}\hspace{2cm}\textsc{100}\end{sideways}
  &
  \begin{overpic}[width=0.3\textwidth]{fig_supp/neuraldiff/100_L1_dinora_reconstruction_diff.jpg}
  \end{overpic}
 &
  \begin{overpic}[width=0.3\textwidth]{fig_supp/neuraldiff/100_L2_dinora_reconstruction_diff.jpg}
  \end{overpic}
  &
  \begin{overpic}[width=0.3\textwidth]{fig_supp/neuraldiff/100_L1L2_dinora_reconstruction_diff.jpg}
  \end{overpic}
  \\
  \begin{sideways}\hspace{2cm}\textsc{150}\end{sideways}
  &
   \begin{overpic}[width=0.3\textwidth]{fig_supp/neuraldiff/150_L1_dinora_reconstruction_diff.jpg}
  \end{overpic}
 &
  \begin{overpic}[width=0.3\textwidth]{fig_supp/neuraldiff/150_L2_dinora_reconstruction_diff.jpg}
  \end{overpic}
  &
  \begin{overpic}[width=0.3\textwidth]{fig_supp/neuraldiff/150_L1L2_dinora_reconstruction_diff.jpg}
  \end{overpic}
  \\
  \begin{sideways}\hspace{2cm}\textsc{200}\end{sideways}
  &
  \begin{overpic}[width=0.3\textwidth]{fig_supp/neuraldiff/200_L1_dinora_reconstruction_diff.jpg}
  \end{overpic}
 &
  \begin{overpic}[width=0.3\textwidth]{fig_supp/neuraldiff/200_L2_dinora_reconstruction_diff.jpg}
  \end{overpic}
  &
  \begin{overpic}[width=0.3\textwidth]{fig_supp/neuraldiff/200_L1L2_dinora_reconstruction_diff.jpg}
  \end{overpic}
 \end{tabular}
 \vspace{-3mm}
%  \caption{Dinora}
  \caption{Subject F - Type V}
  \label{fig:neuraldiff_6}
  \vspace{-6mm}
\end{figure*}

\begin{figure*}
 \contourlength{0.1em}%
 \centering
 \hspace*{-4.5mm}%
  \begin{tabular}{l@{\;}c@{\;}c@{\;}c}
 & \textsc{L1} & \textsc{L2} & \textsc{L1L2} 
  \\
   \begin{sideways}\hspace{1cm}\textsc{50}\end{sideways}
  &
  \begin{overpic}[width=0.3\textwidth]{fig_supp/neuraldiff/50_L1_brownfemale_reconstruction_diff.jpg}
  \end{overpic}
 &
  \begin{overpic}[width=0.3\textwidth]{fig_supp/neuraldiff/50_L2_brownfemale_reconstruction_diff.jpg}
  \end{overpic}
  &
  \begin{overpic}[width=0.3\textwidth]{fig_supp/neuraldiff/50_L1L2_brownfemale_reconstruction_diff.jpg}
  \end{overpic}
  \\
  \begin{sideways}\hspace{1cm}\textsc{100}\end{sideways}
  &
  \begin{overpic}[width=0.3\textwidth]{fig_supp/neuraldiff/100_L1_brownfemale_reconstruction_diff.jpg}
  \end{overpic}
 &
  \begin{overpic}[width=0.3\textwidth]{fig_supp/neuraldiff/100_L2_brownfemale_reconstruction_diff.jpg}
  \end{overpic}
  &
  \begin{overpic}[width=0.3\textwidth]{fig_supp/neuraldiff/100_L1L2_brownfemale_reconstruction_diff.jpg}
  \end{overpic}
  \\
  \begin{sideways}\hspace{1cm}\textsc{150}\end{sideways}
  &
   \begin{overpic}[width=0.3\textwidth]{fig_supp/neuraldiff/150_L1_brownfemale_reconstruction_diff.jpg}
  \end{overpic}
 &
  \begin{overpic}[width=0.3\textwidth]{fig_supp/neuraldiff/150_L2_brownfemale_reconstruction_diff.jpg}
  \end{overpic}
  &
  \begin{overpic}[width=0.3\textwidth]{fig_supp/neuraldiff/150_L1L2_brownfemale_reconstruction_diff.jpg}
  \end{overpic}
  \\
  \begin{sideways}\hspace{1cm}\textsc{200}\end{sideways}
  &
  \begin{overpic}[width=0.3\textwidth]{fig_supp/neuraldiff/200_L1_brownfemale_reconstruction_diff.jpg}
  \end{overpic}
 &
  \begin{overpic}[width=0.3\textwidth]{fig_supp/neuraldiff/200_L2_brownfemale_reconstruction_diff.jpg}
  \end{overpic}
  &
  \begin{overpic}[width=0.3\textwidth]{fig_supp/neuraldiff/200_L1L2_brownfemale_reconstruction_diff.jpg}
  \end{overpic}
 \end{tabular}
 \vspace{-3mm}
%  \caption{brownfemale}
  \caption{Subject G - Type V}
  \label{fig:neuraldiff_7}
  \vspace{-6mm}
\end{figure*}

\begin{figure*}
 \contourlength{0.1em}%
 \centering
 \hspace*{-4.5mm}%
  \begin{tabular}{l@{\;}c@{\;}c@{\;}c}
 & \textsc{L1} & \textsc{L2} & \textsc{L1L2} 
  \\
   \begin{sideways}\hspace{1cm}\textsc{50}\end{sideways}
  &
  \begin{overpic}[width=0.3\textwidth]{fig_supp/neuraldiff/50_L1_darkmale_reconstruction_diff.jpg}
  \end{overpic}
 &
  \begin{overpic}[width=0.3\textwidth]{fig_supp/neuraldiff/50_L2_darkmale_reconstruction_diff.jpg}
  \end{overpic}
  &
  \begin{overpic}[width=0.3\textwidth]{fig_supp/neuraldiff/50_L1L2_darkmale_reconstruction_diff.jpg}
  \end{overpic}
  \\
  \begin{sideways}\hspace{1cm}\textsc{100}\end{sideways}
  &
  \begin{overpic}[width=0.3\textwidth]{fig_supp/neuraldiff/100_L1_darkmale_reconstruction_diff.jpg}
  \end{overpic}
 &
  \begin{overpic}[width=0.3\textwidth]{fig_supp/neuraldiff/100_L2_darkmale_reconstruction_diff.jpg}
  \end{overpic}
  &
  \begin{overpic}[width=0.3\textwidth]{fig_supp/neuraldiff/100_L1L2_darkmale_reconstruction_diff.jpg}
  \end{overpic}
  \\
  \begin{sideways}\hspace{1cm}\textsc{150}\end{sideways}
  &
   \begin{overpic}[width=0.3\textwidth]{fig_supp/neuraldiff/150_L1_darkmale_reconstruction_diff.jpg}
  \end{overpic}
 &
  \begin{overpic}[width=0.3\textwidth]{fig_supp/neuraldiff/150_L2_darkmale_reconstruction_diff.jpg}
  \end{overpic}
  &
  \begin{overpic}[width=0.3\textwidth]{fig_supp/neuraldiff/150_L1L2_darkmale_reconstruction_diff.jpg}
  \end{overpic}
  \\
  \begin{sideways}\hspace{1cm}\textsc{200}\end{sideways}
  &
  \begin{overpic}[width=0.3\textwidth]{fig_supp/neuraldiff/200_L1_darkmale_reconstruction_diff.jpg}
  \end{overpic}
 &
  \begin{overpic}[width=0.3\textwidth]{fig_supp/neuraldiff/200_L2_darkmale_reconstruction_diff.jpg}
  \end{overpic}
  &
  \begin{overpic}[width=0.3\textwidth]{fig_supp/neuraldiff/200_L1L2_darkmale_reconstruction_diff.jpg}
  \end{overpic}
 \end{tabular}
 \vspace{-3mm}
%  \caption{darkmale}
  \caption{Subject H - Type VI}
  \label{fig:neuraldiff_8}
  \vspace{-6mm}
\end{figure*}
