# Supplementary material for: Estimation of Spectral Biophysical Skin Properties from Captured RGB Albedo
Source: arXiv:2201.10695 source file (2022-01-26)
Supplement: Supplementary file 2 [file neuralreconstruction.tex]

\section{Neural Network Structure Effect on Multiple Reconstructions}
In Figure~\ref{fig:neuralreconstruction_1} - Figure~\ref{fig:neuralreconstruction_8}, we show the neural reconstruction results for the skin albedo of each subject. We compare the results of different network structures (50, 100, 150, 200 hidden layer dimensions) and different loss functions. As explained in the main paper Section 5.2.3, the total loss consists of three parts: $L = L_{param}+ \alpha L_{albedo} + \beta L_{albedo}'$. In this Supplemental, we use $L_1$ to denote that the $L_1$ difference is applied on all three losses; we use $L_2$ to denote that the $L_2$ difference is applied on all three losses; $L_1L_2$ means that we use the $L_1$ difference on $L_{albedo}$ and $L_{albedo}'$, and the $L_2$ difference on $L_{param}$. The reconstruction losses on all faces are reported in Table~\ref{tab:error}. The loss is only computed on the skin regions. Please see the albedo reconstruction figures for the masks that cover the non-skin regions. As shown in Table~\ref{tab:error}, using 200 hidden layer dimension with the $L_1L_2$ strategy (200 $L_1L_2$) achieves the highest accuracy overall. However we observed that the network with 150 hidden layer dimension produces an equivalent level of errors visually as 200. In practice the smaller structure (150 $L_1 L_2$) is preferable.

\begin{figure*}
 \contourlength{0.1em}%
 \centering
 \hspace*{-4.5mm}%
  \begin{tabular}{l@{\;}c@{\;}c@{\;}c@{\;}c}
 & \textsc{Input} & \textsc{L1} & \textsc{L2} & \textsc{L1L2} 
  \\
   \begin{sideways}\hspace{2cm}\textsc{50}\end{sideways}
    &
  \begin{overpic}[width=0.25\textwidth]{fig_supp/neuralreconstruction/50_L1_laure_reconstruction.jpg}
  \end{overpic}
  &
  \begin{overpic}[width=0.25\textwidth]{fig_supp/neuralreconstruction/50_L1_laure_reconstruction.jpg}
  \end{overpic}
 &
  \begin{overpic}[width=0.25\textwidth]{fig_supp/neuralreconstruction/50_L2_laure_reconstruction.jpg}
  \end{overpic}
  &
  \begin{overpic}[width=0.25\textwidth]{fig_supp/neuralreconstruction/50_L1L2_laure_reconstruction.jpg}
  \end{overpic}
  \\
  \begin{sideways}\hspace{2cm}\textsc{100}\end{sideways}
    &
  \begin{overpic}[width=0.25\textwidth]{fig_supp/neuralreconstruction/100_L1_laure_reconstruction.jpg}
  \end{overpic}
  &
  \begin{overpic}[width=0.25\textwidth]{fig_supp/neuralreconstruction/100_L1_laure_reconstruction.jpg}
  \end{overpic}
 &
  \begin{overpic}[width=0.25\textwidth]{fig_supp/neuralreconstruction/100_L2_laure_reconstruction.jpg}
  \end{overpic}
  &
  \begin{overpic}[width=0.25\textwidth]{fig_supp/neuralreconstruction/100_L1L2_laure_reconstruction.jpg}
  \end{overpic}
  \\
  \begin{sideways}\hspace{2cm}\textsc{150}\end{sideways}
   &
   \begin{overpic}[width=0.25\textwidth]{fig_supp/neuralreconstruction/150_L1_laure_reconstruction.jpg}
  \end{overpic}
  &
   \begin{overpic}[width=0.25\textwidth]{fig_supp/neuralreconstruction/150_L1_laure_reconstruction.jpg}
  \end{overpic}
 &
  \begin{overpic}[width=0.25\textwidth]{fig_supp/neuralreconstruction/150_L2_laure_reconstruction.jpg}
  \end{overpic}
  &
  \begin{overpic}[width=0.25\textwidth]{fig_supp/neuralreconstruction/150_L1L2_laure_reconstruction.jpg}
  \end{overpic}
  \\
  \begin{sideways}\hspace{2cm}\textsc{200}\end{sideways}
  &
  \begin{overpic}[width=0.25\textwidth]{fig_supp/neuralreconstruction/200_L1_laure_reconstruction.jpg}
  \end{overpic}
  &
  \begin{overpic}[width=0.25\textwidth]{fig_supp/neuralreconstruction/200_L1_laure_reconstruction.jpg}
  \end{overpic}
 &
  \begin{overpic}[width=0.25\textwidth]{fig_supp/neuralreconstruction/200_L2_laure_reconstruction.jpg}
  \end{overpic}
  &
  \begin{overpic}[width=0.25\textwidth]{fig_supp/neuralreconstruction/200_L1L2_laure_reconstruction.jpg}
  \end{overpic}
 \end{tabular}
 \vspace{-3mm}
%  \caption{Laure}
  \caption{Subject A - Type I}
  \label{fig:neuralreconstruction_1}
  \vspace{-6mm}
\end{figure*}

\begin{figure*}
 \contourlength{0.1em}%
 \centering
 \hspace*{-4.5mm}%
   \begin{tabular}{l@{\;}c@{\;}c@{\;}c@{\;}c}
 & \textsc{Input} & \textsc{L1} & \textsc{L2} & \textsc{L1L2} 
  \\
   \begin{sideways}\hspace{1cm}\textsc{50}\end{sideways}
    &
  \begin{overpic}[width=0.25\textwidth]{fig_supp/neuralreconstruction/50_L1_whitefemale_reconstruction.jpg}
  \end{overpic}
  &
  \begin{overpic}[width=0.25\textwidth]{fig_supp/neuralreconstruction/50_L1_whitefemale_reconstruction.jpg}
  \end{overpic}
 &
  \begin{overpic}[width=0.25\textwidth]{fig_supp/neuralreconstruction/50_L2_whitefemale_reconstruction.jpg}
  \end{overpic}
  &
  \begin{overpic}[width=0.25\textwidth]{fig_supp/neuralreconstruction/50_L1L2_whitefemale_reconstruction.jpg}
  \end{overpic}
  \\
  \begin{sideways}\hspace{1cm}\textsc{100}\end{sideways}
    &
  \begin{overpic}[width=0.25\textwidth]{fig_supp/neuralreconstruction/100_L1_whitefemale_reconstruction.jpg}
  \end{overpic}
  &
  \begin{overpic}[width=0.25\textwidth]{fig_supp/neuralreconstruction/100_L1_whitefemale_reconstruction.jpg}
  \end{overpic}
 &
  \begin{overpic}[width=0.25\textwidth]{fig_supp/neuralreconstruction/100_L2_whitefemale_reconstruction.jpg}
  \end{overpic}
  &
  \begin{overpic}[width=0.25\textwidth]{fig_supp/neuralreconstruction/100_L1L2_whitefemale_reconstruction.jpg}
  \end{overpic}
  \\
  \begin{sideways}\hspace{1cm}\textsc{150}\end{sideways}
    &
   \begin{overpic}[width=0.25\textwidth]{fig_supp/neuralreconstruction/150_L1_whitefemale_reconstruction.jpg}
  \end{overpic}
  &
   \begin{overpic}[width=0.25\textwidth]{fig_supp/neuralreconstruction/150_L1_whitefemale_reconstruction.jpg}
  \end{overpic}
 &
  \begin{overpic}[width=0.25\textwidth]{fig_supp/neuralreconstruction/150_L2_whitefemale_reconstruction.jpg}
  \end{overpic}
  &
  \begin{overpic}[width=0.25\textwidth]{fig_supp/neuralreconstruction/150_L1L2_whitefemale_reconstruction.jpg}
  \end{overpic}
  \\
  \begin{sideways}\hspace{1cm}\textsc{200}\end{sideways}
   &
  \begin{overpic}[width=0.25\textwidth]{fig_supp/neuralreconstruction/200_L1_whitefemale_reconstruction.jpg}
  \end{overpic}
  &
  \begin{overpic}[width=0.25\textwidth]{fig_supp/neuralreconstruction/200_L1_whitefemale_reconstruction.jpg}
  \end{overpic}
 &
  \begin{overpic}[width=0.25\textwidth]{fig_supp/neuralreconstruction/200_L2_whitefemale_reconstruction.jpg}
  \end{overpic}
  &
  \begin{overpic}[width=0.25\textwidth]{fig_supp/neuralreconstruction/200_L1L2_whitefemale_reconstruction.jpg}
  \end{overpic}
 \end{tabular}
 \vspace{-3mm}
%  \caption{whitefemale}
  \caption{Subject B - Type I}
  \label{fig:neuralreconstruction_2}
  \vspace{-6mm}
\end{figure*}

\begin{figure*}
 \contourlength{0.1em}%
 \centering
 \hspace*{-4.5mm}%
  \begin{tabular}{l@{\;}c@{\;}c@{\;}c@{\;}c}
 & \textsc{Input} & \textsc{L1} & \textsc{L2} & \textsc{L1L2} 
  \\
  \begin{sideways}\hspace{2cm}\textsc{50}\end{sideways}
  &
  \begin{overpic}[width=0.25\textwidth]{fig_supp/neuralreconstruction/50_L1_ronald_reconstruction.jpg}
  \end{overpic}
  &
  \begin{overpic}[width=0.25\textwidth]{fig_supp/neuralreconstruction/50_L1_ronald_reconstruction.jpg}
  \end{overpic}
 &
  \begin{overpic}[width=0.25\textwidth]{fig_supp/neuralreconstruction/50_L2_ronald_reconstruction.jpg}
  \end{overpic}
  &
  \begin{overpic}[width=0.25\textwidth]{fig_supp/neuralreconstruction/50_L1L2_ronald_reconstruction.jpg}
  \end{overpic}
  \\
  \begin{sideways}\hspace{2cm}\textsc{100}\end{sideways}
  &
  \begin{overpic}[width=0.25\textwidth]{fig_supp/neuralreconstruction/100_L1_ronald_reconstruction.jpg}
  \end{overpic}
  &
  \begin{overpic}[width=0.25\textwidth]{fig_supp/neuralreconstruction/100_L1_ronald_reconstruction.jpg}
  \end{overpic}
 &
  \begin{overpic}[width=0.25\textwidth]{fig_supp/neuralreconstruction/100_L2_ronald_reconstruction.jpg}
  \end{overpic}
  &
  \begin{overpic}[width=0.25\textwidth]{fig_supp/neuralreconstruction/100_L1L2_ronald_reconstruction.jpg}
  \end{overpic}
  \\
  \begin{sideways}\hspace{2cm}\textsc{150}\end{sideways}
   &
   \begin{overpic}[width=0.25\textwidth]{fig_supp/neuralreconstruction/150_L1_ronald_reconstruction.jpg}
  \end{overpic}
  &
   \begin{overpic}[width=0.25\textwidth]{fig_supp/neuralreconstruction/150_L1_ronald_reconstruction.jpg}
  \end{overpic}
 &
  \begin{overpic}[width=0.25\textwidth]{fig_supp/neuralreconstruction/150_L2_ronald_reconstruction.jpg}
  \end{overpic}
  &
  \begin{overpic}[width=0.25\textwidth]{fig_supp/neuralreconstruction/150_L1L2_ronald_reconstruction.jpg}
  \end{overpic}
  \\
  \begin{sideways}\hspace{2cm}\textsc{200}\end{sideways}
  &
  \begin{overpic}[width=0.25\textwidth]{fig_supp/neuralreconstruction/200_L1_ronald_reconstruction.jpg}
  \end{overpic}
  &
  \begin{overpic}[width=0.25\textwidth]{fig_supp/neuralreconstruction/200_L1_ronald_reconstruction.jpg}
  \end{overpic}
 &
  \begin{overpic}[width=0.25\textwidth]{fig_supp/neuralreconstruction/200_L2_ronald_reconstruction.jpg}
  \end{overpic}
  &
  \begin{overpic}[width=0.25\textwidth]{fig_supp/neuralreconstruction/200_L1L2_ronald_reconstruction.jpg}
  \end{overpic}
 \end{tabular}
 \vspace{-3mm}
%  \caption{Ronald}
  \caption{Subject C - Type II}
  \label{fig:neuralreconstruction_3}
  \vspace{-6mm}
\end{figure*}

\begin{figure*}
 \contourlength{0.1em}%
 \centering
 \hspace*{-4.5mm}%
 \begin{tabular}{l@{\;}c@{\;}c@{\;}c@{\;}c}
 & \textsc{Input} & \textsc{L1} & \textsc{L2} & \textsc{L1L2} 
  \\
   \begin{sideways}\hspace{2cm}\textsc{50}\end{sideways}
    &
  \begin{overpic}[width=0.25\textwidth]{fig_supp/neuralreconstruction/50_L1_tony_reconstruction.jpg}
  \end{overpic}
  &
  \begin{overpic}[width=0.25\textwidth]{fig_supp/neuralreconstruction/50_L1_tony_reconstruction.jpg}
  \end{overpic}
 &
  \begin{overpic}[width=0.25\textwidth]{fig_supp/neuralreconstruction/50_L2_tony_reconstruction.jpg}
  \end{overpic}
  &
  \begin{overpic}[width=0.25\textwidth]{fig_supp/neuralreconstruction/50_L1L2_tony_reconstruction.jpg}
  \end{overpic}
  \\
  \begin{sideways}\hspace{2cm}\textsc{100}\end{sideways}
  &
  \begin{overpic}[width=0.25\textwidth]{fig_supp/neuralreconstruction/100_L1_tony_reconstruction.jpg}
  \end{overpic}
  &
  \begin{overpic}[width=0.25\textwidth]{fig_supp/neuralreconstruction/100_L1_tony_reconstruction.jpg}
  \end{overpic}
 &
  \begin{overpic}[width=0.25\textwidth]{fig_supp/neuralreconstruction/100_L2_tony_reconstruction.jpg}
  \end{overpic}
  &
  \begin{overpic}[width=0.25\textwidth]{fig_supp/neuralreconstruction/100_L1L2_tony_reconstruction.jpg}
  \end{overpic}
  \\
  \begin{sideways}\hspace{2cm}\textsc{150}\end{sideways}
  &
   \begin{overpic}[width=0.25\textwidth]{fig_supp/neuralreconstruction/150_L1_tony_reconstruction.jpg}
  \end{overpic}
  &
   \begin{overpic}[width=0.25\textwidth]{fig_supp/neuralreconstruction/150_L1_tony_reconstruction.jpg}
  \end{overpic}
 &
  \begin{overpic}[width=0.25\textwidth]{fig_supp/neuralreconstruction/150_L2_tony_reconstruction.jpg}
  \end{overpic}
  &
  \begin{overpic}[width=0.25\textwidth]{fig_supp/neuralreconstruction/150_L1L2_tony_reconstruction.jpg}
  \end{overpic}
  \\
  \begin{sideways}\hspace{2cm}\textsc{200}\end{sideways}
   &
  \begin{overpic}[width=0.25\textwidth]{fig_supp/neuralreconstruction/200_L1_tony_reconstruction.jpg}
  \end{overpic}
  &
  \begin{overpic}[width=0.25\textwidth]{fig_supp/neuralreconstruction/200_L1_tony_reconstruction.jpg}
  \end{overpic}
 &
  \begin{overpic}[width=0.25\textwidth]{fig_supp/neuralreconstruction/200_L2_tony_reconstruction.jpg}
  \end{overpic}
  &
  \begin{overpic}[width=0.25\textwidth]{fig_supp/neuralreconstruction/200_L1L2_tony_reconstruction.jpg}
  \end{overpic}
 \end{tabular}
 \vspace{-3mm}
%  \caption{Tony}
  \caption{Subject D - Type III}
  \label{fig:neuralreconstruction_4}
  \vspace{-6mm}
\end{figure*}

\begin{figure*}
 \contourlength{0.1em}%
 \centering
 \hspace*{-4.5mm}%
 \begin{tabular}{l@{\;}c@{\;}c@{\;}c@{\;}c}
 & \textsc{Input} & \textsc{L1} & \textsc{L2} & \textsc{L1L2} 
  \\
    \begin{sideways}\hspace{2cm}\textsc{50}\end{sideways}
    &
  \begin{overpic}[width=0.25\textwidth]{fig_supp/neuralreconstruction/50_L1_yaser_reconstruction.jpg}
  \end{overpic}
  &
  \begin{overpic}[width=0.25\textwidth]{fig_supp/neuralreconstruction/50_L1_yaser_reconstruction.jpg}
  \end{overpic}
 &
  \begin{overpic}[width=0.25\textwidth]{fig_supp/neuralreconstruction/50_L2_yaser_reconstruction.jpg}
  \end{overpic}
  &
  \begin{overpic}[width=0.25\textwidth]{fig_supp/neuralreconstruction/50_L1L2_yaser_reconstruction.jpg}
  \end{overpic}
  \\
  \begin{sideways}\hspace{2cm}\textsc{100}\end{sideways}
  &
  \begin{overpic}[width=0.25\textwidth]{fig_supp/neuralreconstruction/100_L1_yaser_reconstruction.jpg}
  \end{overpic}
  &
  \begin{overpic}[width=0.25\textwidth]{fig_supp/neuralreconstruction/100_L1_yaser_reconstruction.jpg}
  \end{overpic}
 &
  \begin{overpic}[width=0.25\textwidth]{fig_supp/neuralreconstruction/100_L2_yaser_reconstruction.jpg}
  \end{overpic}
  &
  \begin{overpic}[width=0.25\textwidth]{fig_supp/neuralreconstruction/100_L1L2_yaser_reconstruction.jpg}
  \end{overpic}
  \\
  \begin{sideways}\hspace{2cm}\textsc{150}\end{sideways}
  &
   \begin{overpic}[width=0.25\textwidth]{fig_supp/neuralreconstruction/150_L1_yaser_reconstruction.jpg}
  \end{overpic}
  &
   \begin{overpic}[width=0.25\textwidth]{fig_supp/neuralreconstruction/150_L1_yaser_reconstruction.jpg}
  \end{overpic}
 &
  \begin{overpic}[width=0.25\textwidth]{fig_supp/neuralreconstruction/150_L2_yaser_reconstruction.jpg}
  \end{overpic}
  &
  \begin{overpic}[width=0.25\textwidth]{fig_supp/neuralreconstruction/150_L1L2_yaser_reconstruction.jpg}
  \end{overpic}
  \\
  \begin{sideways}\hspace{2cm}\textsc{200}\end{sideways}
  &
  \begin{overpic}[width=0.25\textwidth]{fig_supp/neuralreconstruction/200_L1_yaser_reconstruction.jpg}
  \end{overpic}
  &
  \begin{overpic}[width=0.25\textwidth]{fig_supp/neuralreconstruction/200_L1_yaser_reconstruction.jpg}
  \end{overpic}
 &
  \begin{overpic}[width=0.25\textwidth]{fig_supp/neuralreconstruction/200_L2_yaser_reconstruction.jpg}
  \end{overpic}
  &
  \begin{overpic}[width=0.25\textwidth]{fig_supp/neuralreconstruction/200_L1L2_yaser_reconstruction.jpg}
  \end{overpic}
 \end{tabular}
 \vspace{-3mm}
%  \caption{Yaser}
  \caption{Subject E - Type IV}
  \label{fig:neuralreconstruction_5}
  \vspace{-6mm}
\end{figure*}

\begin{figure*}
 \contourlength{0.1em}%
 \centering
 \hspace*{-4.5mm}%
  \begin{tabular}{l@{\;}c@{\;}c@{\;}c@{\;}c}
 & \textsc{Input} & \textsc{L1} & \textsc{L2} & \textsc{L1L2} 
  \\
   \begin{sideways}\hspace{2cm}\textsc{50}\end{sideways}
     &
  \begin{overpic}[width=0.25\textwidth]{fig_supp/neuralreconstruction/50_L1_dinora_reconstruction.jpg}
  \end{overpic}
  &
  \begin{overpic}[width=0.25\textwidth]{fig_supp/neuralreconstruction/50_L1_dinora_reconstruction.jpg}
  \end{overpic}
 &
  \begin{overpic}[width=0.25\textwidth]{fig_supp/neuralreconstruction/50_L2_dinora_reconstruction.jpg}
  \end{overpic}
  &
  \begin{overpic}[width=0.25\textwidth]{fig_supp/neuralreconstruction/50_L1L2_dinora_reconstruction.jpg}
  \end{overpic}
  \\
  \begin{sideways}\hspace{2cm}\textsc{100}\end{sideways}
    &
  \begin{overpic}[width=0.25\textwidth]{fig_supp/neuralreconstruction/100_L1_dinora_reconstruction.jpg}
  \end{overpic}
  &
  \begin{overpic}[width=0.25\textwidth]{fig_supp/neuralreconstruction/100_L1_dinora_reconstruction.jpg}
  \end{overpic}
 &
  \begin{overpic}[width=0.25\textwidth]{fig_supp/neuralreconstruction/100_L2_dinora_reconstruction.jpg}
  \end{overpic}
  &
  \begin{overpic}[width=0.25\textwidth]{fig_supp/neuralreconstruction/100_L1L2_dinora_reconstruction.jpg}
  \end{overpic}
  \\
  \begin{sideways}\hspace{2cm}\textsc{150}\end{sideways}
    &
   \begin{overpic}[width=0.25\textwidth]{fig_supp/neuralreconstruction/150_L1_dinora_reconstruction.jpg}
  \end{overpic}
  &
   \begin{overpic}[width=0.25\textwidth]{fig_supp/neuralreconstruction/150_L1_dinora_reconstruction.jpg}
  \end{overpic}
 &
  \begin{overpic}[width=0.25\textwidth]{fig_supp/neuralreconstruction/150_L2_dinora_reconstruction.jpg}
  \end{overpic}
  &
  \begin{overpic}[width=0.25\textwidth]{fig_supp/neuralreconstruction/150_L1L2_dinora_reconstruction.jpg}
  \end{overpic}
  \\
  \begin{sideways}\hspace{2cm}\textsc{200}\end{sideways}
    &
  \begin{overpic}[width=0.25\textwidth]{fig_supp/neuralreconstruction/200_L1_dinora_reconstruction.jpg}
  \end{overpic}
  &
  \begin{overpic}[width=0.25\textwidth]{fig_supp/neuralreconstruction/200_L1_dinora_reconstruction.jpg}
  \end{overpic}
 &
  \begin{overpic}[width=0.25\textwidth]{fig_supp/neuralreconstruction/200_L2_dinora_reconstruction.jpg}
  \end{overpic}
  &
  \begin{overpic}[width=0.25\textwidth]{fig_supp/neuralreconstruction/200_L1L2_dinora_reconstruction.jpg}
  \end{overpic}
 \end{tabular}
 \vspace{-3mm}
%  \caption{Dinora}
  \caption{Subject F - Type V}
  \label{fig:neuralreconstruction_6}
  \vspace{-6mm}
\end{figure*}

\begin{figure*}
 \contourlength{0.1em}%
 \centering
 \hspace*{-4.5mm}%
 \begin{tabular}{l@{\;}c@{\;}c@{\;}c@{\;}c}
 & \textsc{Input} & \textsc{L1} & \textsc{L2} & \textsc{L1L2} 
  \\
   \begin{sideways}\hspace{1cm}\textsc{50}\end{sideways}
     &
  \begin{overpic}[width=0.25\textwidth]{fig_supp/neuralreconstruction/50_L1_brownfemale_reconstruction.jpg}
  \end{overpic}
  &
  \begin{overpic}[width=0.25\textwidth]{fig_supp/neuralreconstruction/50_L1_brownfemale_reconstruction.jpg}
  \end{overpic}
 &
  \begin{overpic}[width=0.25\textwidth]{fig_supp/neuralreconstruction/50_L2_brownfemale_reconstruction.jpg}
  \end{overpic}
  &
  \begin{overpic}[width=0.25\textwidth]{fig_supp/neuralreconstruction/50_L1L2_brownfemale_reconstruction.jpg}
  \end{overpic}
  \\
  \begin{sideways}\hspace{1cm}\textsc{100}\end{sideways}
    &
  \begin{overpic}[width=0.25\textwidth]{fig_supp/neuralreconstruction/100_L1_brownfemale_reconstruction.jpg}
  \end{overpic}
  &
  \begin{overpic}[width=0.25\textwidth]{fig_supp/neuralreconstruction/100_L1_brownfemale_reconstruction.jpg}
  \end{overpic}
 &
  \begin{overpic}[width=0.25\textwidth]{fig_supp/neuralreconstruction/100_L2_brownfemale_reconstruction.jpg}
  \end{overpic}
  &
  \begin{overpic}[width=0.25\textwidth]{fig_supp/neuralreconstruction/100_L1L2_brownfemale_reconstruction.jpg}
  \end{overpic}
  \\
  \begin{sideways}\hspace{1cm}\textsc{150}\end{sideways}
    &
   \begin{overpic}[width=0.25\textwidth]{fig_supp/neuralreconstruction/150_L1_brownfemale_reconstruction.jpg}
  \end{overpic}
  &
   \begin{overpic}[width=0.25\textwidth]{fig_supp/neuralreconstruction/150_L1_brownfemale_reconstruction.jpg}
  \end{overpic}
 &
  \begin{overpic}[width=0.25\textwidth]{fig_supp/neuralreconstruction/150_L2_brownfemale_reconstruction.jpg}
  \end{overpic}
  &
  \begin{overpic}[width=0.25\textwidth]{fig_supp/neuralreconstruction/150_L1L2_brownfemale_reconstruction.jpg}
  \end{overpic}
  \\
  \begin{sideways}\hspace{1cm}\textsc{200}\end{sideways}
    &
  \begin{overpic}[width=0.25\textwidth]{fig_supp/neuralreconstruction/200_L1_brownfemale_reconstruction.jpg}
  \end{overpic}
  &
  \begin{overpic}[width=0.25\textwidth]{fig_supp/neuralreconstruction/200_L1_brownfemale_reconstruction.jpg}
  \end{overpic}
 &
  \begin{overpic}[width=0.25\textwidth]{fig_supp/neuralreconstruction/200_L2_brownfemale_reconstruction.jpg}
  \end{overpic}
  &
  \begin{overpic}[width=0.25\textwidth]{fig_supp/neuralreconstruction/200_L1L2_brownfemale_reconstruction.jpg}
  \end{overpic}
 \end{tabular}
 \vspace{-3mm}
%  \caption{brownfemale}
  \caption{Subject G - Type V}
  \label{fig:neuralreconstruction_7}
  \vspace{-6mm}
\end{figure*}

\begin{figure*}
 \contourlength{0.1em}%
 \centering
 \hspace*{-4.5mm}%
   \begin{tabular}{l@{\;}c@{\;}c@{\;}c@{\;}c}
 & \textsc{Input} & \textsc{L1} & \textsc{L2} & \textsc{L1L2} 
  \\
   \begin{sideways}\hspace{1cm}\textsc{50}\end{sideways}
     &
  \begin{overpic}[width=0.25\textwidth]{fig_supp/neuralreconstruction/50_L1_darkmale_reconstruction.jpg}
  \end{overpic}
  &
  \begin{overpic}[width=0.25\textwidth]{fig_supp/neuralreconstruction/50_L1_darkmale_reconstruction.jpg}
  \end{overpic}
 &
  \begin{overpic}[width=0.25\textwidth]{fig_supp/neuralreconstruction/50_L2_darkmale_reconstruction.jpg}
  \end{overpic}
  &
  \begin{overpic}[width=0.25\textwidth]{fig_supp/neuralreconstruction/50_L1L2_darkmale_reconstruction.jpg}
  \end{overpic}
  \\
  \begin{sideways}\hspace{1cm}\textsc{100}\end{sideways}
    &
  \begin{overpic}[width=0.25\textwidth]{fig_supp/neuralreconstruction/100_L1_darkmale_reconstruction.jpg}
  \end{overpic}
  &
  \begin{overpic}[width=0.25\textwidth]{fig_supp/neuralreconstruction/100_L1_darkmale_reconstruction.jpg}
  \end{overpic}
 &
  \begin{overpic}[width=0.25\textwidth]{fig_supp/neuralreconstruction/100_L2_darkmale_reconstruction.jpg}
  \end{overpic}
  &
  \begin{overpic}[width=0.25\textwidth]{fig_supp/neuralreconstruction/100_L1L2_darkmale_reconstruction.jpg}
  \end{overpic}
  \\
  \begin{sideways}\hspace{1cm}\textsc{150}\end{sideways}
    &
   \begin{overpic}[width=0.25\textwidth]{fig_supp/neuralreconstruction/150_L1_darkmale_reconstruction.jpg}
  \end{overpic}
  &
   \begin{overpic}[width=0.25\textwidth]{fig_supp/neuralreconstruction/150_L1_darkmale_reconstruction.jpg}
  \end{overpic}
 &
  \begin{overpic}[width=0.25\textwidth]{fig_supp/neuralreconstruction/150_L2_darkmale_reconstruction.jpg}
  \end{overpic}
  &
  \begin{overpic}[width=0.25\textwidth]{fig_supp/neuralreconstruction/150_L1L2_darkmale_reconstruction.jpg}
  \end{overpic}
  \\
  \begin{sideways}\hspace{1cm}\textsc{200}\end{sideways}
   &
  \begin{overpic}[width=0.25\textwidth]{fig_supp/neuralreconstruction/200_L1_darkmale_reconstruction.jpg}
  \end{overpic}
  &
  \begin{overpic}[width=0.25\textwidth]{fig_supp/neuralreconstruction/200_L1_darkmale_reconstruction.jpg}
  \end{overpic}
 &
  \begin{overpic}[width=0.25\textwidth]{fig_supp/neuralreconstruction/200_L2_darkmale_reconstruction.jpg}
  \end{overpic}
  &
  \begin{overpic}[width=0.25\textwidth]{fig_supp/neuralreconstruction/200_L1L2_darkmale_reconstruction.jpg}
  \end{overpic}
 \end{tabular}
 \vspace{-3mm}
%  \caption{darkmale}
  \caption{Subject H - Type VI}
  \label{fig:neuralreconstruction_8}
  \vspace{-6mm}
\end{figure*}
