# Supplementary material for: Estimation of Spectral Biophysical Skin Properties from Captured RGB Albedo
Source: arXiv:2201.10695 source file (2022-01-26)
Supplement: Supplementary file 8 [file table.tex]

\begin{table*}
    \centering
    \begin{tabular}{ |c|c|c|c|c|c|c|c|c|c| } 
\hline
& Subject A
& Subject B
& Subject C
& Subject D
& Subject E
& Subject F
& Subject G
& Subject H
& Average over subjects\\
 \hline
 50 L1 
 & 0.0097
 & 0.0219
 & 0.0117
 &  0.01624
& 0.0138
& 0.0085
& 0.0107
& 0.0035
& 0.0120\\
\hline
 50 L2
 & 0.0060
& 0.0077
& 0.0037
 & 0.0037
& 0.0034
& 0.0049
& 0.0042

& 0.0030
& 0.0046\\
\hline
 50 L1L2
 & 0.0060
 & 0.0077
 & 0.0037
 & 0.0037
& 0.0034
& 0.0049
& 0.0042
& 0.0030
&  0.0046\\
\hline
 100 L1 
 & 0.0047
 & 0.0053
 & 0.0023
 & 0.0021
& 0.0022
& 0.0030
& 0.0053
& 0.0015
& 0.0033\\
\hline
 100 L2 
 & 0.0055
 & 0.0059
 & 0.0033
 & 0.0035
& 0.0030
& 0.0038
& 0.0037
& 0.0027
& 0.0039\\
\hline
100 L1L2 
& 0.0044
& 0.0057
& 0.0022
& 0.0022
& 0.0023
& 0.0038
& 0.0050
& 0.0017
& 0.0034\\
\hline
150 L1
& 0.0040
& 0.0047
& 0.0021
& 0.0027
& 0.0022
& 0.0020
& 0.0050
& 0.0013
& 0.0030\\
\hline
150 L2 
& 0.0063
& 0.0056
& 0.0027
& 0.0025
& 0.0024
& 0.0029
& 0.0034
& 0.0020
& 0.0035\\
\hline
150 L1L2
& 0.0037
& 0.0049
& 0.0021
& 0.0023
& 0.0023
& 0.0030
& 0.0033
& 0.0015
& 0.0029\\
\hline
200 L1
& 0.0041
& 0.0047
& 0.0024
& 0.0030
& 0.0028
& 0.0017
& 0.0029
& 0.0013
& 0.0029\\
\hline
200 L2 
& 0.0061
& 0.0060
& 0.0028
& 0.0025
& 0.0023
& 0.0028
& 0.0030
& 0.0017
& 0.0034\\
\hline
200 L1L2
& 0.0039
& 0.0047
& 0.0017
& 0.0014
& 0.0014
& 0.0022
& 0.0033
& 0.0009
& 0.0024\\
\hline
\end{tabular}
\caption{We compare different network structure and loss function combinations and report the average absolute difference between the reconstruction and the input albedo. The metric is only computed on the unmasked region. Please see the albedo reconstruction figures for the masked and unmasked regions. The metric shows that using 200 hidden layer dimension and $L_1$ albedo losses and $L_2$ parameter loss (200 $L_1L_2$) achieves the highest accuracy overall. However we observed that the network with 150 hidden layer dimension produces an equivalent level of errors visually as 200 neurons. In practice the smaller structure (150 $L_1 L_2$) is more preferable.}
\label{tab:error}
\end{table*}
